# Supplementary material for: Kleister: A novel task for Information Extraction involving Long Documents with Complex Layout
Source: arXiv:2003.02356 source file (2020-03-06)
Supplement: Supplementary file 1 [file the-appendix.tex]

\documentclass[11pt,a4paper]{article}
\usepackage[hyperref]{acl2020}
\usepackage{times}
\usepackage{latexsym}

\usepackage{microtype}

\input{extras}
\input{preamble}

\begin{document}

\input{appendix}

\end{document}
